# Supplementary material for: Synergistic Scheduling of Learning and Allocation of Tasks in Human-Robot Teams
Source: arXiv:2203.07478 source file (2022-07-07)
Supplement: Supplementary file 2 [file 9_appendix.tex]

\appendix 
\section{Planning}
\subsection{Special Case: Deterministic Preconditions}
Consider the common case of a deterministic precondition model.
% We relax the requirement for a human to be available at all times.
% However, their availability is known a priori.
In this secction, we show that this problem can be transformed into the \textit{Set Cover}~\cite{vazirani2013approximation} problem.

For a skill $\pi$, given its precondition and the set $U$ of tasks to be solved, define its coverage  as: $S_{\pi} = \{\tau : \rho_{\pi}(\tau) = 1, \tau \in U\}$.
We seek to \textit{cover} all the tasks using some learned skill or by asking for human help.
Assume $c_{fail} \geq c_{hum}$ so the optimal strategy is to delegate to a human if the robot cannot handle a task.
For every task $\tau_i$, we introduce a set $S_i = S_{\pi_i}$ where $\pi_i$ is the skill to be learned on that task and a set $T_i = \{\tau_i\}$ corresponding to human help.
We associate a cost of $c_{demo}'(i)$ with $S_i$ and $c_{hum}'(i)$ with $T_i$.
Our planning problem can now be restated in terms of the set cover problem: \textit{Find a minimum cost collection of sets $C \subseteq \{S_1,\cdots,S_n\} \cup \{T_1,\cdots,T_n\}$ that covers (solves) all the given tasks.}

\begin{theorem}
There exists a polynomial-time algorithm for this special case that is $\log(n)$  sub-optimal, where $n$ is the number of tasks.
\label{th:set_cover}
\end{theorem}
\textit{Proof Sketch:}
As shown above, we can solve the ADL problem by first converting it to the set cover problem in polynomial time and solving the latter.
The greedy algorithm~\cite{vazirani2013approximation} for solving the set cover problem is $\log(n)$ sub-optimal, which also provides a polynomial-time $\log(n)$ sub-optimal algorithm for ADL.

In theorem ~\ref{th:set_cover}, we proved that ADL can be solved in polynomial-time with bounded cost.
Here, we provide such an algorithm.
As stated in the proof, the key idea is to translate the ADL problem into a set cover problem and apply the greedy algorithm for the same.

\begin{algorithm}[!ht]
    \begin{algorithmic}[1]
        \Procedure{Coverage}{$a, j$}
            \If{$a == a_{demo}$}
                \State \Return{$S_j$}
            \Else
                \State \Return{$\{j\}$}
            \EndIf
        \EndProcedure
        \Procedure{GetGreedyPlan}{$C, i$}
            \State{Initialize $\eta$ with $a_{rob}$}
            \State{$\hat{S}_j \leftarrow \textsc{Coverage}(a_{demo}, j) - C\ \forall j \geq i$} 
            \State{$\hat{T}_j \leftarrow \textsc{Coverage}(a_{hum}, j) - C\ \forall j \geq i$}  
            \While {$C \neq U$}
                \State{Initialize $c[\cdot,\cdot]$ with $\infty$}
                \State{$c[a_{demo}, j] \leftarrow \frac{c_{demo} - c_{rob}}{|\hat{S}_j|}\ \forall\ j \geq i$}
                \State{$c[a_{hum}, j] \leftarrow \frac{c_{hum} - c_{rob}}{|\hat{T}_j|}\ \forall\ j \geq i$}
                \State{$a^*, j^* \leftarrow \argmin c$ \Comment{Best action}}
                \State{$\eta[j^*] \leftarrow a^*$}
                \State{$S^* \leftarrow \textsc{Coverage}(a^*, j^*)$}
                \State{$C \leftarrow C \cup S^*$ \Comment{Tasks covered so far}}
                \State{$\hat{S}_j \leftarrow \hat{S}_j - S^*, \hat{T}_j \leftarrow \hat{T}_j - S^*\  \forall\ j \geq i$}
            \EndWhile
            \State \Return $\eta$
        \EndProcedure
        \Procedure{Main}{}
            \State{$i \leftarrow 1$}
            \State{$C \leftarrow \{\}$}
            \While{\textsc{Not done}}
                \State{$\eta \leftarrow \textsc{GetGreedyPlan}(C, i)$}
                \State{$a \leftarrow \eta[i]$}
                \State{$C \leftarrow $ \textsc{Execute}(a)}
                \State{$i \leftarrow i + 1$}
            \EndWhile
        \EndProcedure
    \end{algorithmic}
    \caption{Polynomial-time planner for deterministic preconditions.}
    \label{alg:greedy-planner}
\end{algorithm}

\section{Additional Experimental Details}
\subsection{Block Insertion}
\begin{figure}[h]
    \centering
    \subfloat[][]{
        \includegraphics[align=c,width=0.5\columnwidth]{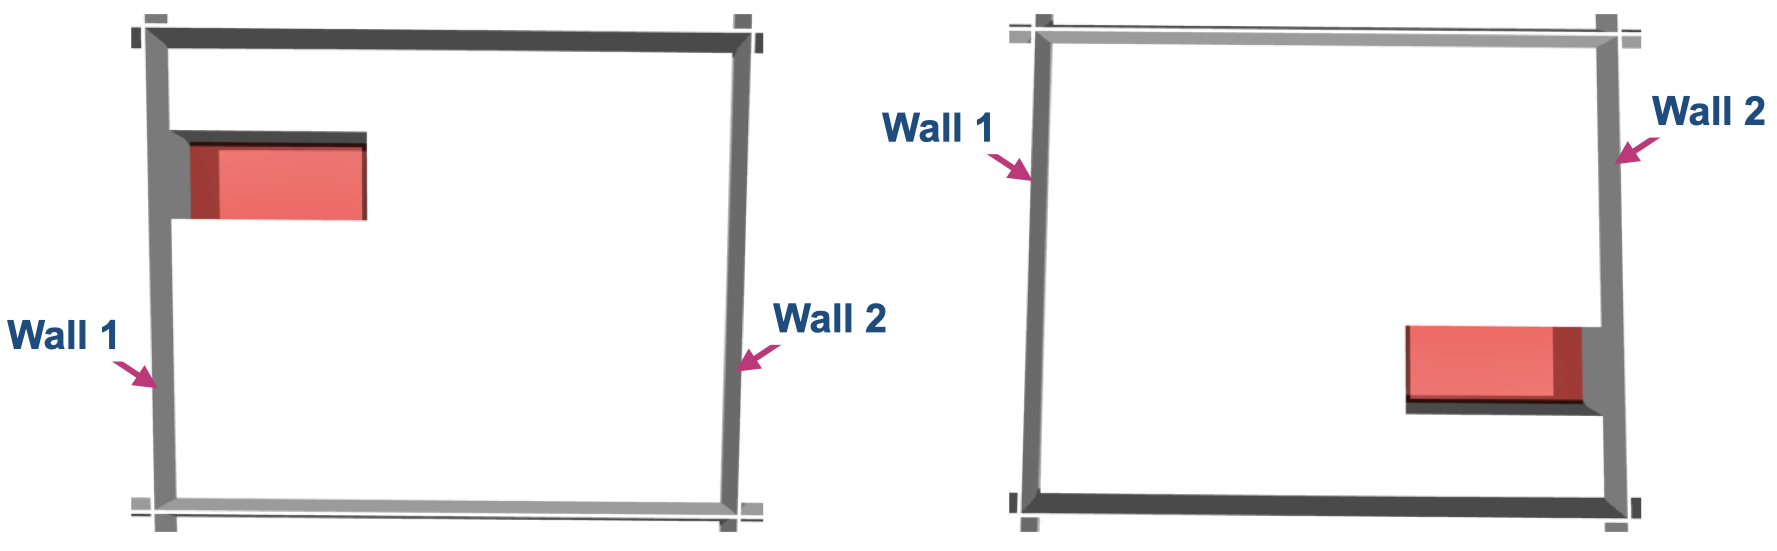}
        \includegraphics[align=c,width=0.5\columnwidth]{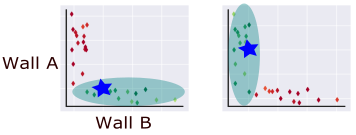}
    }
    % \subfloat[][]{
        % \includegraphics[align=c,width=0.3\columnwidth]{preconditions.png}
    % }
    \caption{(a) We show two different block insertion tasks. In both tasks, the slot location is uncertain, because of which, the robot needs to first press against a neighboring wall to localize. The final insertion policy depends on the locations of walls around a slot. (left) Policy localizes against wall 1 as it is the closest. (right) Policy localizes against wall 2 as it is the closest. (b) The green ellipses indicate the preconditions of skills learned on two block insertion tasks (slot marked with a star). (left) The slot is located close to wall B. Consequently, the learned skill only generalizes to slots close to wall B. (right) The slot is located close to wall A. Consequently, the learned skill only generalizes to slots close to wall A. }
    \label{fig:peg_tasks_and_preconds}
\end{figure}

\begin{figure}[h]
    \centering
    \subfloat[][]{
        \includegraphics[width=0.15\columnwidth]{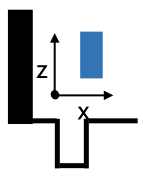}
    }
    \subfloat[][]{
        \includegraphics[width=0.15\columnwidth]{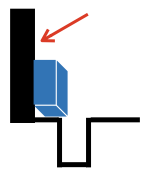}
    }
    \subfloat[][]{
        \includegraphics[width=0.15\columnwidth]{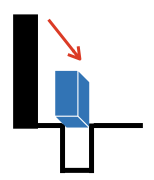}
    }   
    \subfloat[][]{
        \includegraphics[width=0.15\columnwidth]{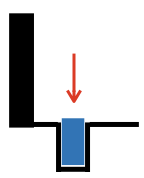}
    }
    \caption{Shown here is a side-view of a 4-step block insertion strategy. The block is shown in blue, the wall next to the slot is shown in solid black and the red arrow points along the force vector applied on the board by the robot. The robot knows the location of the slot with respect to the wall and hence first pushes against it to reduce uncertainty in the x direction.}
    \label{fig:insertion_strategy}
\end{figure}

\begin{figure}[!h]
    \centering
    \subfloat[][]{
        \includegraphics[align=b,width=0.5\columnwidth]{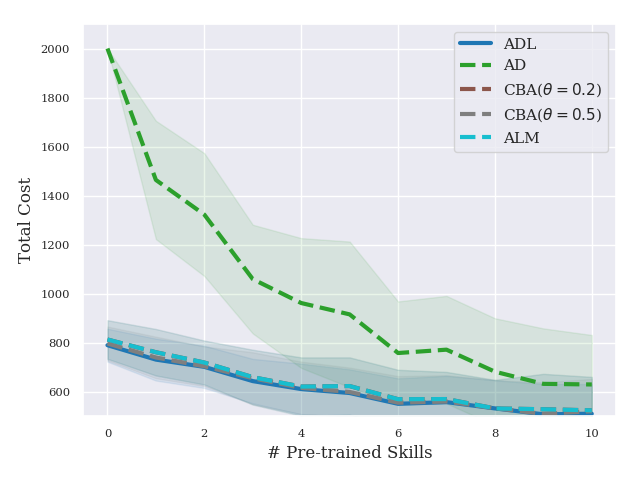}
        }
    \subfloat[][]{
        \includegraphics[align=b,width=0.5\columnwidth]{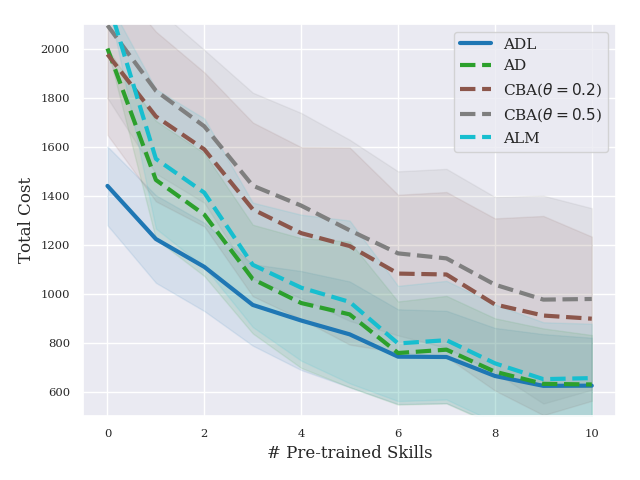}
    }
    \caption{We compare ADL with baselines in two settings. In the first, $c_{demo} < c_{hum} < c_{rob} + c_{fail}$ while, $c_{hum} < c_{rob} + c_{fail} < c_{demo} $ in the latter (we use $c_{rob} = 10$ and $c_{hum} = c_{fail} = 100$ in both) (a) $c_{demo} = 90$: The cost-optimal strategy is to ask for demos if the robot is not confident. Both CBA and ALM perform as well as ADL in this setting. (b) $c_{demo} = 300$: It is important to plan ahead to be able to minimize the number of demos. ADL performs substantially better than baselines in this setting.}
    \label{fig:peg_insertion_additional_plots}
\end{figure}

\textbf{Precondition Prediction Model}
We generate a set of 100 tasks from the same 4 environments.
For 30 tasks out of these, we learn block insertion policies using Relative Entropy Policy Search (REPS)~\cite{peters2010relative}.
These 30 skills are evaluated on all the 100 tasks to  generate success  binary labels.
Using this data we train a 2-layer fully connected neural network as the precondition prediction model.
Given training and test task features $\tau_{train}$ and $\tau_{test}$, we feed $\tau_{train} - \tau_{test}$ as input to the model to encode translational invariance.

\subsection{Real World Peg Insertion}
\begin{figure}[h!]
    \centering
    \subfloat[][]{
        \includegraphics[width=0.26\columnwidth]{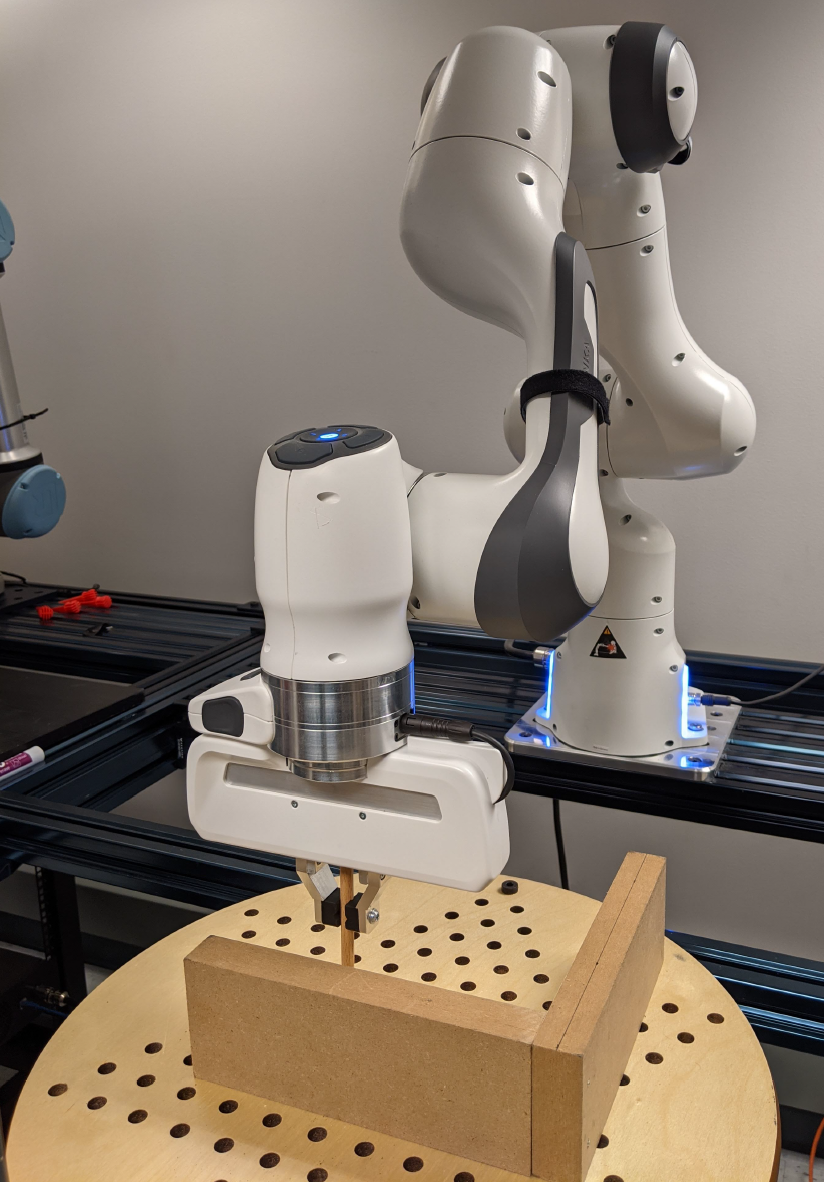}
    }
    \subfloat[][]{
        \includegraphics[width=0.5\columnwidth]{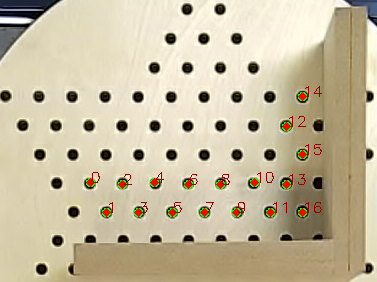}
    }
    \caption{(a) Peg insertion under uncertainty in the real world (b) Shown here is an overhead image of the task setup. In our experiments, we focused on the holes (highlighted in red) close to the two wooden walls so that the robot could always use one of the walls to localize the peg with respect to the target hole. The task-id corresponding to each hole is written next to it.}
    \label{fig:real_tasks}
\end{figure}

We do a qualitative evaluation of our approach on peg insertion in the real world using the 7 DoF Franka Emika Panda arm.
In our approximate model, we assume that there is always only one hole in the task area and each new task is a different set of walls and hole.
However, in the real world we use  a single Chinese checkers board with many holes on it.
Each task here is fully specified by its location on the board.
From a set of 17 tasks, we create 5 sets of 10 tasks each for evaluating our approach.

The results from our experiment are summarized in in table \ref{table:results_real}.
In task set 1 (table ~\ref{table:results_real}), all the tasks are close to the bottom wall and hence can be solved using the same skill.
The precondition prediction model is able to capture this relationship, which is why ADL asks for only 1 demo and doesn’t delegate to a human.
In task set 2 (table ~\ref{table:results_real}), tasks 12 and 14 lie close to the right wall and hence need a skill different from the one that can solve the other 8 tasks in that set.
Because the precondition model is able to predict this (a) it does not ask the robot to attempt these two tasks and (b) it delegates them to the human as it is not cost-effective to seek additional demos for just two tasks.

\begin{table}[h!]
\centering
    \begin{tabular}{c|l}
         & Order of Tasks \\
         \midrule
       1 & 0, 1, 2, 3, 4, 5, 6, 7, 8, 9 \\
       2 & 0, 1, 2, 12, 3, 4, 14, 5, 6, 7 \\
       3 & 1, 0, 2, 12, 3, 4, 14, 5, 6, 7 \\
       4 & 1, 3, 2, 12, 0, 4, 14, 5, 6, 7 \\
       5 & 1, 3, 5, 7, 0, 12, 4, 14, 2, 6
    \end{tabular}
    \quad \quad
    \begin{tabular}{ccc}
                 & \#demo & \# hum \\ \midrule
      1   & 1 & 0  \\
      2   & 1 & 2  \\
      3   & 1 & 3  \\
      4   & 1 & 4  \\
      5   & 2 & 2  \\               
    \end{tabular}
    \caption{We assume $c_{rob} = 10, c_{hum} = 100, c_{fail} = 100, c_{demo} = 300$. Our parameterized preconditions model learned in simulation transfers to the real world as it is able to capture the relative distances of walls from the hole.}
\label{table:results_real}
\end{table}

\subsection{Lego Stacking}
\begin{table}
\centering
    \begin{tabular}{lcccc}\toprule
                             & Total Cost          &   \# demo    & \# hum  & \# fail      \\ \midrule
        ADL           & \textbf{856} ($\pm$ 120.9)      & 1.2 ($\pm$ 0.4)    & 4.2 ($\pm$ 1.7)  & 1.5 ($\pm$ 1)  \\
        % D            & 1000 ($\pm$ 0)        & 0 ($\pm$ 0)    & 10 ($\pm$ 0)  & 0 ($\pm$ 0)  \\
        % A             & 1460 ($\pm$ 227.1)      & 4.9 ($\pm$ 1.5)    & 0 ($\pm$ 0) & 3.8 ($\pm$ 1.5)
        AD            & 1000 ($\pm$ 0)        & 0 ($\pm$ 0)    & 10 ($\pm$ 0)  & 0 ($\pm$ 0)  \\
        CBA ($\theta=0.5$)             & 1306 ($\pm$ 207.2)      & 5.4 ($\pm$ 1.2)    & 0 ($\pm$ 0) & 1.8 ($\pm$ 1.5) \\
        ALM            & 1100 ($\pm$ 0)        & 0 ($\pm$ 0)    & 0 ($\pm$ 0)  & 10 ($\pm$ 0) 
        
      \end{tabular}
    \caption{We report the mean and standard deviation of the results averaged over 10 different planning problems with 10 tasks each. Baselines ALM, AD and CBA($\theta=0.5$) cost $28.5\%$, $16.8\%$ and $52.6\%$ more than ADL as they don't plan ahead.  We use $c_{rob} = 10$, $c_{hum} = 100$, $c_{fail} = 100$,  $c_{demo} = 200$ and no skill pretraining.}
\label{table:results1}
\end{table}
\textbf{Skills:} The following skills are executed in sequence-
\begin{enumerate}
\item \textbf{Pickup:} Picks up the part given a grasp location.
\item \textbf{Place and Wiggle:} Places the part at the target location and pushes it down while perturbing the part randomly to align it with the studs on the base plate.
For all parts, except the smallest ones, this step alone is not sufficient for firm stacking as it only ensures stacking within a small region around the grasp.
\item \textbf{Robust Tapping:} Pushes down on the part at different locations to make sure that the part is stacked firmly.
\end{enumerate}

\textbf{Precondition Prediction Model:} We capture 10 images of each of the 15 tasks, along with a bounding box around the part and the grasp location.  After training skills for each of the resulting 150 tasks in our coverage-based simulation, we evaluate them on all the tasks to generate binary success labels
Using this data we train a 2-layer fully connected neural network as the precondition prediction model.
Given training and test task features $\tau_{train}$ and $\tau_{test}$, we feed $[\tau_{train},  \tau_{test}]$ as input to the model.
